# Supplementary material for: Semi-global approach for propagation of the time-dependent Schr\"odinger equation for time-dependent and nonlinear problems
Source: arXiv:1611.06707 ancillary file (2017-05-01)
Supplement: Supplementary file 1 [file f_error.pdf]

# Estimation of the error of the direct computation of

$$\tilde{f}_m(z, t)$$

Ido Schaefer

April 30, 2017

The function to be computed is (Sec. 3.4.2):

$$\tilde{f}_m(z, t) \equiv \begin{cases} \frac{m!}{z^m} \left[ \exp(zt) - \sum_{j=0}^{m-1} \frac{(zt)^j}{j!} \right] & z \neq 0 \\ t^m & z = 0 \end{cases} \quad m = 0, 1, \dots \quad (1)$$

In order to compute it in the case of  $z \neq 0$ , we define:

$$\bar{f}_m(z) \equiv \frac{m!}{z^m} \left[ \exp(z) - \sum_{j=0}^{m-1} \frac{z^j}{j!} \right] \quad z \neq 0 \quad (2)$$

We have:

$$\tilde{f}_m(z, t) = t^m \bar{f}_m(zt), \quad z \neq 0 \quad (3)$$

Let us define, for convenience:

$$\bar{z} = zt \quad (4)$$

$\bar{f}_m(\bar{z})$  can be computed by the following recursion:

$$\bar{f}_0(\bar{z}) = \exp(\bar{z}) \quad (5)$$

$$\bar{f}_m(\bar{z}) = \frac{m}{\bar{z}} [\bar{f}_{m-1}(\bar{z}) - 1], \quad m > 0 \quad (6)$$

This procedure suffers from roundoff errors. Let us estimate the order of the relative error for  $\bar{f}_m(\bar{z})$ .

Let us denote the computed  $\bar{f}_m(\bar{z})$  by  $\bar{f}_m^C(\bar{z})$ . We can write:

$$\bar{f}_m^C(\bar{z}) = \frac{m}{\bar{z}} [\bar{f}_{m-1}^C(\bar{z}) - 1 + \tau_{m-1}] \quad (7)$$

where  $\tau_j$  denotes the roundoff error of the computation of  $\bar{f}_j^C(\bar{z}) - 1$ . By applying the recurrence relation (7) successively, we finally obtain the following expression:

$$\bar{f}_m^C(\bar{z}) = \frac{m!}{\bar{z}^m} \left[ \exp(\bar{z}) - \sum_{j=0}^{m-1} \frac{\bar{z}^j}{j!} (1 - \tau_j) \right] \quad (8)$$

The absolute error of the computation is given by

$$E_m(\bar{z}) = |\bar{f}_m^C(\bar{z}) - \bar{f}_m(\bar{z})| = \frac{m!}{|\bar{z}|^m} \sum_{j=0}^{m-1} \frac{|\bar{z}|^j}{j!} |\tau_j| = m! \sum_{j=0}^{m-1} \frac{|\tau_j|}{j! |\bar{z}|^{m-j}} \quad (9)$$

The relative error is

$$E_m^{rel}(\bar{z}) = \frac{m!}{|\bar{f}_m(\bar{z})|} \sum_{j=0}^{m-1} \frac{|\tau_j|}{j! |\bar{z}|^{m-j}} \quad (10)$$

Let us denote the computational machine precision (`eps` in MATLAB) by  $\epsilon$ . The order of

$\tau_j$  can be estimated in the following way:

$$\tau_j \sim \begin{cases} |\bar{f}_j^C(\bar{z})| \epsilon, & |\bar{f}_j^C(\bar{z})| > 1 \\ \epsilon, & |\bar{f}_j^C(\bar{z})| < 1 \end{cases} \quad (11)$$

If  $\bar{z} \ll 1$ , then  $\bar{f}_j^C(\bar{z})$  is close to 1, and  $\tau_j$  can be estimated by  $\epsilon$ . We obtain the following estimation for the relative error:

$$E_m^{rel}(\bar{z}) \sim m! \epsilon \sum_{j=0}^{m-1} \frac{1}{j! |\bar{z}|^{m-j}} \quad (12)$$

Since  $\bar{z} \ll 1$ , the magnitude of the error can be estimated by the largest term in the sum, with  $j = 0$ . We obtain:

$$E_m^{rel}(\bar{z}) \sim \frac{m!}{|\bar{z}|^m} \epsilon \quad (13)$$

The roundoff error may be significant even when the condition  $\bar{z} \ll 1$  is not satisfied. For instance, let us take  $\bar{z} = 1$ . In this case, all the  $\bar{f}_m(\bar{z})$ 's are of order of 1. Thus, we can give a rough estimation of (10) by

$$E_m^{rel}(\bar{z}) \sim m! \epsilon \quad (14)$$

For a double precision,  $\epsilon \sim 10^{-16}$ . If we choose  $m = 12$ , we obtain  $E_m^{rel}(\bar{z}) \sim 10^{-7}$ . For  $m = 15$ , we obtain  $E_m^{rel}(\bar{z}) \sim 10^{-4}$ .

The Taylor expansion is not a good alternative in such a case. It involves many expansion terms, and may also become unstable for larger  $\bar{z}$ . Possible solutions are:

1. Performing the computation of  $\bar{f}_m(\bar{z})$  in higher precision than the double precision; the computation is a scalar computation, and the extra memory required is negligible. The other computations in the algorithm needn't be performed in the higher

precision.

2. Using another alternative computation from the Taylor approximation—performing a numerical integration of the integrals which led to the functions  $\tilde{f}_m(z, t)$ ,

$$\tilde{f}_m(z, t) = m \int_0^t \exp[z(t - \tau)] \tau^{m-1} d\tau = mt^m \int_0^1 \exp[\bar{z}(1 - y)] y^{m-1} dy = t^m \bar{f}_m(\bar{z}) \quad (15)$$

with

$$\bar{f}_m(\bar{z}) = m \int_0^1 \exp[\bar{z}(1 - y)] y^{m-1} dy \quad (16)$$

It is recommended to use a Legendre integration.
